# Supplementary material for: Time-integration of Gaussian variational approximation for the magnetic Schr\"odinger equation
Source: arXiv:2504.03407 source file (2025-04-04)
Supplement: Supplementary file 1 [file old-stuff-appendix.tex]

%%%%%%%%%%%%%%%%%%%%%%%%%%%%%%%%%%%%%%%%%%%%%%%%%
FROM APPENDIX
%%%%%%%%%%%%%%%%%%%%%%%%%%%%%%%%%%%%%%%%%%%%%%%%%



\begin{lemma}\label{Lemma:intPotdtAbsGWP}
    With a sufficiently smooth potential \(\somePot\colon\bbR\times\Rd\to\bbR\) and a \GWP \(\vsol\) we have
    \begin{align}
        &\intRd\somePot(t, x)\pt\abs{\vsol(t, x)}^2\dx \nonumber\\
        &\qquad\qquad= 
        \frac{\scp}{2}\tr\mean[\Big]{\hessian{\somePot}\big(\ReC - \mean{\jacobian{\mgPot}}\big)\ImCinv}
        +
        \mean{\nabla W}^T\vel, \label{eq:intPotdtAbsGWP}
    \end{align}
    were \(\hessian{\somePot}\) denotes the Hessian matrix w.r.t. \(x\) of \(\somePot\).
\end{lemma}
\begin{proof}
    For the derivative \(\pt\abs{\vsol(t, x)}^2\) we get
    \begin{align}
        \pt\abs{\vsol(t, x)}^2 
        &= 
        \abs{\vsol(t, x)}^2\bigg(\frac{2}{\scp}(x-\pos(t))^T
        \big(
            \ReC(t) - \mean{\jacobian{\mgPot}^T(t)}
        \big)\ImC(t)(x-\pos(t)) \nonumber\\
        &\qquad\qquad\qquad 
        + \frac{2}{\scp}(x-\pos(t))^T\ImC(t)\vel(t) - \tr(\ReC(t))\bigg). \label{eq:timeDerv_absGWP}
    \end{align} 
    To simplify the notation we ignore the dependence on \(t\) in the following. Inserting~\eqref{eq:timeDerv_absGWP} into~\eqref{eq:intPotdtAbsGWP} leads to
    \begin{align}
        &\intRd\somePot(x)\pt\abs{\vsol(x)}^2\dx \nonumber\\
        &\qquad
        = \frac{2}{\scp}\intRd\somePot(x)(x - \pos)^T\big(
            \ReC - \mean{\jacobian{\mgPot}}^T
        \big)\ImC(x - \pos)\abs{\vsol(x)}^2\dx \nonumber\\
        &\qquad\quad
        + \frac{2}{\scp}\intRd\somePot(x)(x - \pos)^T\ImC\vel\abs{\vsol(x)}^2\dx 
        - \mean{\somePot}\tr(\ReC) \nonumber\\
        &\qquad
        = \frac{\scp}{2}\tr\mean[\Big]{\hessian{\somePot}\big(\ReC - \mean{\jacobian{\mgPot}}\big)\ImCinv}
        + \mean{\nabla W}^T\vel,
    \end{align}
    where we have used in the last equality Lemma~\ref{aux:lemma:integral-1} with \(D = \ReC - \mean{\jacobian{\mgPot}}^T\) and \(\tr(\jacobian{\mgPot}) = \Div \mgPot = 0\) for the first integral and 
    \begin{align}\label{eq:gradAbsGWP}
        \nabla\abs{\vsol(x)}^2 = -\frac{2}{\scp}\ImC(x-\pos)\abs{\vsol(x)}^2
    \end{align}
    with partial integration for the second integral.
\end{proof}

\begin{lemma}\label{aux:lemma:integral-1}
    With a smooth potential \(\somePot\colon\bbR\times\bbR^d\to\bbR\) and matrix $D\in\bbC^{\dim\times \dim}$ independent of \(x\) it holds
    \begin{align}
        &\frac{2}{\scp}\intRd \somePot(x)(x-\pos)^TD\IC(x-\pos)\abs{\vsol(x)}^2\dx \\
        &\qquad\qquad= 
        \frac{\scp}{2}\mean{\tr(\hessian{\somePot}D^T\ImCinv} 
        + \mean{\somePot}\tr D . \label{aux:eq:integral_1}
    \end{align}
    % where $\widetilde{D} = D^T\ImCinv$ and
    % \begin{equation}
    %     \left(\auxDervMgPot{\widetilde{D}}(x)\right)_i \da \sum\limits_{j, k = 1}^d\ptl_k\ptl_j \mgPot_i(x)\widetilde{d}_{j k} 
    %     = \tr\left(\hessian{\mgPot_i}\widetilde{D}\right).
    % \end{equation}
\end{lemma}
\begin{proof}
    By using
    \begin{align}
        \nabla\abs{\vsol(x)}^2 = -\frac{2}{\scp}\ImC(x-\pos)\abs{\vsol(x)}^2
    \end{align}
    combined with two-fold partial integration we get
    \begin{align}
        &\frac{2}{\scp}\intRd \somePot(x)(x-\pos)^TD\IC(x-\pos)\abs{\vsol(x)}^2\dx \\
        &\qquad=
        -\intRd\somePot(x)(x-\pos)^T D \nabla\abs{\vsol(x)}^2\dx \\
        &\qquad= 
        \intRd(\nabla\somePot(x))^T D^T(x-\pos)\abs{\vsol(x)}^2\dx + \mean{W}\tr D \\
        &\qquad=
        -\frac{\scp}{2}\intRd(\nabla\somePot(x))^T D^T\ImCinv\nabla\abs{\vsol(x)}^2\dx + \mean{W}\tr D \\
        &\qquad=
        \frac{\scp}{2}\intRd\tr(\hessian{\somePot}(x)D^T\ImCinv)\abs{\vsol(x)}^2\dx + \mean{W}\tr D ,
    \end{align}
    which proves the statement.
\end{proof}
